# Supplementary material for: Separate versus Pooled Winsorization in Difference-in-Differences: Bias, Efficiency, and Finite-Sample Guarantees
Source: arXiv:2606.15097 source file (2026-11-14)
Supplement: Supplementary file 1 [file appendix_b_quantile_localization.tex]

\subsection{Proof of Lemma~\ref{lem:quantile-localization} (Quantile Localization)}
\label{app:proof-quantile-localization}

Let $u=\log(48/\delta)$ and $A_c=2c^2+\tfrac{8c}{3}$. By assumption,
$m\varepsilon\ge A_cu$. By continuity of $F$,
\[
F(\alpha^-)=\varepsilon-\varepsilon/c,
\quad
F(\alpha^+)=\varepsilon+\varepsilon/c,
\quad
\Prob(X>\beta^-)=\varepsilon+\varepsilon/c,
\quad
\Prob(X>\beta^+)=\varepsilon-\varepsilon/c.
\]
Set $k=\lceil\varepsilon m\rceil$ and $\ell=\lceil(1-\varepsilon)m\rceil$.

Define events
\[
E_1=\{\hat\alpha<\alpha^-\},\ 
E_2=\{\hat\alpha>\alpha^+\},\ 
E_3=\{\hat\beta<\beta^-\},\ 
E_4=\{\hat\beta>\beta^+\}.
\]
We show $\Prob(E_j)\le\delta/48$ for $j=1,\dots,4$.

For $E_1$, with $W_i^-=\1\{X_i\le\alpha^-\}$ and
$p_-=\E(W_i^-)=\varepsilon-\varepsilon/c$,
\[
E_1=\{X_{(k)}<\alpha^-\}\subseteq\{F_m(\alpha^-)\ge\varepsilon\}
\subseteq\{F_m(\alpha^-)-p_-\ge\varepsilon/c\}.
\]
Applying Bernstein inequality (See Lemma~\ref{lem:bernstein-app}) gives
\[
\Prob(E_1)
\le
\exp\!\left(-\frac{m(\varepsilon/c)^2}{2p_-+\tfrac{2}{3}(\varepsilon/c)}\right)
\le
\exp\!\left(-\frac{m(\varepsilon/c)^2}{2\varepsilon+\tfrac{8}{3}(\varepsilon/c)}\right)
\le e^{-u}=\frac{\delta}{48},
\]
where the last step uses $m\varepsilon\ge A_cu$.

For $E_2$, let $p_+=F(\alpha^+)=\varepsilon+\varepsilon/c$. Since
$X_{(k)}>\alpha^+$ implies $F_m(\alpha^+)\le (k-1)/m<\varepsilon$,
\[
E_2\subseteq\{p_+-F_m(\alpha^+)\ge\varepsilon/c\},
\]
and the same Bernstein bound gives $\Prob(E_2)\le\delta/48$.

For $E_3$, define $U_i^-=\1\{X_i>\beta^-\}$,
$r_-=\E(U_i^-)=\varepsilon+\varepsilon/c$. Since
$X_{(\ell)}<\beta^-$ implies $F_m(\beta^-)\ge \ell/m\ge1-\varepsilon$,
\[
E_3\subseteq\{r_--(1-F_m(\beta^-))\ge\varepsilon/c\},
\]
so $\Prob(E_3)\le\delta/48$.

For $E_4$, define $U_i^+=\1\{X_i>\beta^+\}$,
$r_+=\E(U_i^+)=\varepsilon-\varepsilon/c$. Since
$X_{(\ell)}>\beta^+$ implies $F_m(\beta^+)\le(\ell-1)/m<1-\varepsilon$,
\[
E_4\subseteq\{(1-F_m(\beta^+))-r_+\ge\varepsilon/c\},
\]
so $\Prob(E_4)\le\delta/48$.

A union bound yields
\[
\Prob\!\left(
\alpha^-\le\hat\alpha\le\alpha^+,
\ \beta^-\le\hat\beta\le\beta^+
\right)
\ge
1-4\cdot\frac{\delta}{48}
=
1-\frac{\delta}{12},
\]
which proves Lemma~\ref{lem:quantile-localization}. \qed

\begin{lemma}[Bernstein inequality]
\label{lem:bernstein-app}
Let $Z_1,\dots,Z_m$ be independent, mean-zero random variables with
$|Z_i|\le M$ almost surely, and let $v=\sum_{i=1}^m\E(Z_i^2)$. For all
$t>0$,
\[
\Prob\!\left(\sum_{i=1}^m Z_i\ge t\right)
\le
\exp\!\left(-\frac{t^2}{2(v+Mt/3)}\right).
\]
Consequently,
\[
\Prob\!\left(\left|\sum_{i=1}^m Z_i\right|\ge t\right)
\le
2\exp\!\left(-\frac{t^2}{2(v+Mt/3)}\right).
\]
\end{lemma}

\begin{proof}
See, for example, \citet[Theorem~2.8.4]{vershynin2009high}.
\end{proof}

\subsection{Proof of Lemma~\ref{lem:threshold-perturbation} (Threshold Perturbation)}
\label{app:proof-threshold-perturbation}

Let $u=\log(48/\delta)$ and $A_c=2c^2+\tfrac{8c}{3}$.

Define
\[
\mathcal E_{\mathrm{loc}}
=
\{\alpha^-\le\hat\alpha\le\alpha^+,\ \beta^-\le\hat\beta\le\beta^+\}.
\]
By Lemma~\ref{lem:quantile-localization},
$\Prob(\mathcal E_{\mathrm{loc}})\ge1-\delta/12$.

Define also
\[
\mathcal E_{\mathrm{tail}}
=
\left\{F_m(\alpha^+)\le\varepsilon+\frac{2\varepsilon}{c},
1-F_m(\beta^-)\le\varepsilon+\frac{2\varepsilon}{c}\right\}.
\]
Since $F(\alpha^+)=\varepsilon+\varepsilon/c$, applying the Bernstein inequality for
$\1\{X_i\le\alpha^+\}$ gives
\[
\Prob\!\left(F_m(\alpha^+)>\varepsilon+\frac{2\varepsilon}{c}\right)
\le
\exp\!\left(-\frac{m(\varepsilon/c)^2}{2(\varepsilon+\varepsilon/c)+\tfrac{2}{3}(\varepsilon/c)}\right)
\le e^{-u}=\frac{\delta}{48}.
\]
Likewise, because $\Prob(X>\beta^-)=\varepsilon+\varepsilon/c$, Bernstein inequality for
$\1\{X_i>\beta^-\}$ gives
\[
\Prob\!\left(1-F_m(\beta^-)>\varepsilon+\frac{2\varepsilon}{c}\right)
\le\frac{\delta}{48}.
\]
Hence $\Prob(\mathcal E_{\mathrm{tail}})\ge1-\delta/24$ and with
$\mathcal E=\mathcal E_{\mathrm{loc}}\cap\mathcal E_{\mathrm{tail}}$,
\[
\Prob(\mathcal E)\ge1-\frac{\delta}{8}.
\]

On $\mathcal E_{\mathrm{loc}}$, for any $x\in\R$,
\[
|\phi_{\hat\alpha,\hat\beta}(x)-\phi_{\alpha,\beta}(x)|
\le
|\hat\alpha-\alpha|\,\1\{x\le\max(\hat\alpha,\alpha)\}
+
|\hat\beta-\beta|\,\1\{x\ge\min(\hat\beta,\beta)\}.
\]
Averaging over $X_1,\dots,X_m$ and using the fact that
$\max\{\hat\alpha,\alpha\}\le\alpha^+$,
$\min\{\hat\beta,\beta\}\ge\beta^-$ on $\mathcal E_{\mathrm{loc}}$,
\[
|\hat\mu_{\hat\alpha,\hat\beta}-\hat\mu_{\alpha,\beta}|
\le
|\hat\alpha-\alpha|F_m(\alpha^+)
+
|\hat\beta-\beta|\{1-F_m(\beta^-)\}.
\]
On $\mathcal E_{\mathrm{tail}}$, both empirical tail factors are at most
$\varepsilon(1+2/c)$. On $\mathcal E_{\mathrm{loc}}$,
\[
|\hat\alpha-\alpha|\le|\alpha^+-\alpha^-|,
\qquad
|\hat\beta-\beta|\le|\beta^+-\beta^-|.
\]
By Lemma~\ref{lem:quantile-mean-bound},
\[
|\alpha^+-\alpha^-|\le\frac{2\sigma}{\sqrt{\varepsilon(1-1/c)}},
\qquad
|\beta^+-\beta^-|\le\frac{2\sigma}{\sqrt{\varepsilon(1-1/c)}}.
\]
Therefore, on $\mathcal E$,
\[
|\hat\mu_{\hat\alpha,\hat\beta}-\hat\mu_{\alpha,\beta}|
\le
\frac{4(1+2/c)}{\sqrt{1-1/c}}\,\sigma\sqrt{\varepsilon}
:=L_1\sigma\sqrt{\varepsilon},
\]
with $L_1$ depending only on $c$. Hence
\[
\Prob\!\left(
|\hat\mu_{\hat\alpha,\hat\beta}-\hat\mu_{\alpha,\beta}|
>
L_1\sigma\sqrt{\varepsilon}
\right)
\le\Prob(\mathcal E^c)
\le\frac{\delta}{8},
\]
which is \eqref{eq:threshold-perturbation}. \qed

\subsection{Proof of Lemma~\ref{lem:winsor-concentration} (Winsorized Mean Concentration)}
\label{app:proof-winsor-concentration}

Let
\[
Z_i=\phi_{\alpha,\beta}(X_i)-\mu_{\alpha,\beta},
\qquad
\bar Z=\frac{1}{m}\sum_{i=1}^m Z_i
=\hat\mu_{\alpha,\beta}-\mu_{\alpha,\beta}.
\]
Then $Z_1,\dots,Z_m$ are i.i.d., $\E(Z_i)=0$,
$\Var(Z_i)=\Var\{\phi_{\alpha,\beta}(X_i)\}\le\Var(X_i)\le\sigma^2$, and
$|Z_i|\le \beta-\alpha$. We define $M = \beta - \alpha$.
By Lemma~\ref{lem:quantile-mean-bound},
\[
|\alpha-\mu|\le\frac{\sigma}{\sqrt\varepsilon},
\qquad
|\beta-\mu|\le\frac{\sigma}{\sqrt\varepsilon},
\]
so $M\le 2\sigma/\sqrt\varepsilon$.

Apply the two-sided Bernstein bound from Lemma~\ref{lem:bernstein-app}:
\[
\Prob(|\bar Z|\ge t)
\le
2\exp\!\left(-\frac{mt^2}{2(\sigma^2+Mt/3)}\right),\qquad t>0.
\]
Set $u=\log(48/\delta)$ and
\[
t=2\sigma\sqrt{\frac{u}{m}}+\frac{4Mu}{3m}.
\]
Write $t=a+b$ with $a=2\sigma\sqrt{u/m}$ and $b=4Mu/(3m)$. Then
$t^2\ge a^2=4\sigma^2u/m$ and $t^2\ge bt=4Mut/(3m)$. Hence
\[
\frac{mt^2}{2}
\ge
2u\sigma^2+\frac{2uMt}{3},
\qquad\text{so}\qquad
\frac{mt^2}{2(\sigma^2+Mt/3)}\ge u,
\]
so
\[
\Prob(|\bar Z|\ge t)\le 2e^{-u}=\frac{\delta}{24}.
\]

It remains to bound $t$ by $\sigma\sqrt{u/m}$. Since
$m\varepsilon\ge A_cu$ with $A_c=2c^2+\tfrac{8c}{3}$,
\[
\frac{4Mu}{3m}
\le
\frac{8\sigma u}{3m\sqrt\varepsilon}
\le
\frac{8\sigma}{3\sqrt{A_c}}\sqrt{\frac{u}{m}}.
\]
Therefore
\[
t\le\left(2+\frac{8}{3\sqrt{A_c}}\right)\sigma\sqrt{\frac{u}{m}}
:=L_2\sigma\sqrt{\frac{u}{m}},
\]
with $L_2$ depending only on $c$. This proves
\eqref{eq:winsor-concentration}. \qed

\subsection{Proof of Lemma~\ref{lem:winsor-bias}}
\label{app:proof-winsor-bias}

Recall that $\alpha = Q_\varepsilon$, $\beta = Q_{1-\varepsilon}$, and
\[
\mu - \mu_{\alpha,\beta}
=
\E\bigl[(X-\alpha)\1\{X<\alpha\}\bigr]
+
\E\bigl[(X-\beta)\1\{X>\beta\}\bigr].
\]
Therefore
\[
|\mu-\mu_{\alpha,\beta}|
\le
\E\bigl[|X-\alpha|\1\{X<\alpha\}\bigr]
+
\E\bigl[|X-\beta|\1\{X>\beta\}\bigr].
\]
We would separately derive upper bound for the two terms.

\medskip
 For the first term, we
write $|X-\alpha| \le |X-\mu| + |\mu-\alpha|$, so
\[
\E\bigl[|X-\alpha|\1\{X<\alpha\}\bigr]
\le
\E\bigl[|X-\mu|\1\{X<\alpha\}\bigr]
+ |\mu-\alpha|\Prob(X<\alpha).
\]
By Cauchy--Schwarz,
\[
\E\bigl[|X-\mu|\1\{X<\alpha\}\bigr]
\le
\sigma\sqrt{\Prob(X<\alpha)}
\le
\sigma\sqrt{\varepsilon}.
\]
By Lemma~\ref{lem:quantile-mean-bound},
$|\mu-\alpha| \le \sigma/\sqrt{\varepsilon}$, and
$\Prob(X<\alpha)\le\varepsilon$, so
\[
|\mu-\alpha|\Prob(X<\alpha)
\le
\frac{\sigma}{\sqrt{\varepsilon}}\cdot\varepsilon
= \sigma\sqrt{\varepsilon}.
\]
Therefore $\E[|X-\alpha|\1\{X<\alpha\}] \le 2\sigma\sqrt{\varepsilon}$.

\medskip
For the second term, applying
the same argument with $\beta = Q_{1-\varepsilon}$ and
$\Prob(X>\beta)\le\varepsilon$ yields
$\E[|X-\beta|\1\{X>\beta\}] \le 2\sigma\sqrt{\varepsilon}$.

\medskip
\noindent Combining two terms together, 
\[
|\mu_{\alpha,\beta} - \mu|
\le
4\sigma\sqrt{\varepsilon},
\]
which is exactly \eqref{eq:winsor-bias}.

% --------------------------------------------------
%  APPENDIX E: Quantile--mean distance proof
% --------------------------------------------------

\subsection{Proof of Lemma~\ref{lem:quantile-mean-bound}}
\label{app:proof-quantile-mean}

Fix $p\in(0,1)$.
Use the definition of quantile $Q_p = \inf\{x\in\R:F(x)\ge p\}$.

\medskip
\noindent Case (1): If $Q_p \le \mu$,
set $t = \mu - Q_p \ge 0$. Then
\[
p \le \Prob(X\le Q_p) \le \Prob(X\le\mu-t) \le \Prob(|X-\mu|\ge t)
\le \frac{\sigma^2}{t^2},
\]
where the last step is Chebyshev's inequality. Hence $t \le \sigma/\sqrt{p}$.

\medskip
\noindent Case (2): If $Q_p \ge \mu$,
set $t = Q_p - \mu \ge 0$. Then
\[
1-p \le \Prob(X\ge Q_p) \le \Prob(X\ge\mu+t) \le \Prob(|X-\mu|\ge t)
\le \frac{\sigma^2}{t^2},
\]
so $t \le \sigma/\sqrt{1-p}$.

\medskip
\noindent Combining
$|Q_p - \mu| \le \sigma/\sqrt{\min\{p,1-p\}}$. \qed

% --------------------------------------------------
%  APPENDIX F: Pooled balanced impossibility proof
% --------------------------------------------------
