# Supplementary material for: Separate versus Pooled Winsorization in Difference-in-Differences: Bias, Efficiency, and Finite-Sample Guarantees
Source: arXiv:2606.15097 source file (2026-11-14)
Supplement: Supplementary file 3 [file appendix_c_separated_main_proof.tex]

\section{Proof of Theorem~\ref{thm:sep-winsor-mean} (Separate Winsorization)}
\label{app:proof-sep-winsor-main}
In this section, we present the detailed proof of
Theorem~\ref{thm:sep-winsor-mean}. To establish the finite-sample bound for the
proposed separate winsorization algorithm, we adopt the decomposition technique
for the winsorized sample mean from \cite{kock2025winsorized}. In
Section~\ref{app:sep-lemmas}, we first state the supporting lemmas needed for
the proof. We then present the main proof of
Theorem~\ref{thm:sep-winsor-mean} in
Section~\ref{sec:proof-sep-winsor-mean}. Finally, the detailed proofs of the
lemmas stated in Section~\ref{app:sep-lemmas} are provided in
Sections~\ref{app:proof-quantile-localization}--\ref{app:proof-quantile-mean}.
\subsection{Supporting Lemmas for Theorem~\ref{thm:sep-winsor-mean}}
\label{app:sep-lemmas}

This section collects the technical lemmas used to prove
Theorem~\ref{thm:sep-winsor-mean}. 

First, Lemma~\ref{lem:quantile-localization} establishes that the empirical winsorization cutoffs, $\hat{\alpha}$ and $\hat{\beta}$, center around their respective true quantiles, $\alpha$ and $\beta$, with high probability.
\begin{lemma}[Quantile localization]
\label{lem:quantile-localization}
Let $X_1,\dots,X_m$ be i.i.d. with c.d.f. $F \in \mathcal{P}(\sigma^2)$. Fix
$\varepsilon\in(0,1/4)$, $c>1$, $\delta\in(0,1)$,
and assume
\[
m\varepsilon
\;\ge\;
\Bigl(2c^2+\tfrac{8c}{3}\Bigr)\log(48/\delta).
\]
Let $\alpha=Q_\varepsilon$, $\beta=Q_{1-\varepsilon}$, and
$\hat\alpha=X_{(\lceil\varepsilon m\rceil)}$,
$\hat\beta=X_{(\lceil(1-\varepsilon)m\rceil)}$. Define
\[
\alpha^-=Q_{\varepsilon-\varepsilon/c},
\quad
\alpha^+=Q_{\varepsilon+\varepsilon/c},
\quad
\beta^-=Q_{1-\varepsilon-\varepsilon/c},
\quad
\beta^+=Q_{1-\varepsilon+\varepsilon/c}.
\]
Then
\begin{equation}
\label{eq:quantile-localization}
\Prob\!\left(
  \alpha^-\le\hat\alpha\le\alpha^+,
  \;\beta^-\le\hat\beta\le\beta^+
\right)
\;\ge\;
1-\frac{\delta}{12}.
\end{equation}
\end{lemma}

Building on Lemma~\ref{lem:quantile-localization}, Lemma~\ref{lem:threshold-perturbation} establishes that the difference between the empirical winsorized means evaluated at the empirical and population thresholds, $\bigl|\hat\mu_{\hat\alpha,\hat\beta}-\hat\mu_{\alpha,\beta}\bigr|$, is small with high probability.

\begin{lemma}[Threshold perturbation bound]
\label{lem:threshold-perturbation}
Under the same setup as Lemma~\ref{lem:quantile-localization}, there exists
$L_1>0$ depending only on $c$ such that
\begin{equation}
\label{eq:threshold-perturbation}
\Prob\!\left(
  \bigl|\hat\mu_{\hat\alpha,\hat\beta}-\hat\mu_{\alpha,\beta}\bigr|
  > L_1\,\sigma\,\sqrt{\varepsilon}
\right)
\;\le\;
\frac{\delta}{8},
\end{equation}
where $\hat\mu_{\hat\alpha,\hat\beta}$ and $\hat\mu_{\alpha,\beta}$ are the
empirical winsorized means formed with empirical and population thresholds.
\end{lemma}

Next, Lemma~\ref{lem:winsor-concentration} demonstrates that under the same winsorization scheme, the empirical winsorized mean evaluated at the population thresholds concentrates around its expected value with high probability.

\begin{lemma}[Winsorized mean concentration]
\label{lem:winsor-concentration}
Let $X_1,\dots,X_m$ be i.i.d. with mean $\mu$ and
$\Var(X_1)\le\sigma^2$. Let $\alpha=Q_\varepsilon$, $\beta=Q_{1-\varepsilon}$,
$\hat\mu_{\alpha,\beta}=m^{-1}\sum_{i=1}^m\phi_{\alpha,\beta}(X_i)$, and
$\mu_{\alpha,\beta}=\E\{\phi_{\alpha,\beta}(X_1)\}$. If
\[
m\varepsilon
\;\ge\;
\Bigl(2c^2+\tfrac{8c}{3}\Bigr)\log(48/\delta),
\]
then for any $\delta\in(0,1)$,
\begin{equation}
\label{eq:winsor-concentration}
\Prob\!\left(
  \bigl|\hat\mu_{\alpha,\beta}-\mu_{\alpha,\beta}\bigr|
  > L_2\,\sigma\,\sqrt{\frac{\log(48/\delta)}{m}}
\right)
\;\le\;
\frac{\delta}{24},
\end{equation}
for a constant $L_2>0$ depending only on $c$.
\end{lemma}

Next, Lemma~\ref{lem:winsor-bias} provides a deterministic bound on the winsorization bias, guaranteeing that the systematic error introduced by clipping the tails scales at most with the square root of the winsorization level.

\begin{lemma}[Winsorization bias bound]
\label{lem:winsor-bias}
Under the same setup as Lemma~\ref{lem:winsor-concentration},
\begin{equation}
\label{eq:winsor-bias}
\bigl|\mu_{\alpha,\beta}-\mu\bigr|
\;\le\;
4\,\sigma\,\sqrt{\varepsilon}.
\end{equation}
\end{lemma}

Finally, Lemma~\ref{lem:quantile-mean-bound} provides a universal bound on the distance between a population quantile $Q_p$ and the mean $\mu$. This result plays a crucial role in designing our proposed winsorization level.

\begin{lemma}[Quantile--mean distance]
\label{lem:quantile-mean-bound}
Let $X$ be a real-valued random variable with mean $\mu$ and variance
$\sigma^2<\infty$. For $p\in(0,1)$,
\begin{equation}
\label{eq:quantile-mean-bound}
|Q_p-\mu|
\;\le\;
\frac{\sigma}{\sqrt{\min\{p,1-p\}}}.
\end{equation}
\end{lemma}

\subsection{Proof of Theorem~\ref{thm:sep-winsor-mean} }\label{sec:proof-sep-winsor-mean}
\begin{proof}
Set $u_\delta=\log(48/\delta)$ and $A_c=2c^2+\tfrac{8c}{3}$, so
$\varepsilon=A_cu_\delta/n_{\min}$. To derive the concentration bound for $|\hat{\Delta}^{(\mathrm{sep})} - \Delta|$, we will first consider the winsorized sample mean $\hat{\mu}_g^{(\mathrm{sep})}$. For each group $g\in\{0,1\}$, define population thresholds
$\alpha_g=Q_\varepsilon^{(g)}$ and $\beta_g=Q_{1-\varepsilon}^{(g)}$. By the
triangle inequality,
\[
\bigl|\hat\mu_g^{(\mathrm{sep})}-\mu_g\bigr|
\le
\underbrace{\bigl|\hat\mu_{\hat\alpha_g,\hat\beta_g}-\hat\mu_{\alpha_g,\beta_g}\bigr|}_{\text{(I)}}
+
\underbrace{\bigl|\hat\mu_{\alpha_g,\beta_g}-\mu_{\alpha_g,\beta_g}\bigr|}_{\text{(II)}}
+
\underbrace{\bigl|\mu_{\alpha_g,\beta_g}-\mu_g\bigr|}_{\text{(III)}}.
\]
% %Since $n_g\ge n_{\min}$, the assumptions of
% Lemmas~\ref{lem:quantile-localization}--\ref{lem:winsor-concentration} hold in
% each group.
Lemma~\ref{lem:threshold-perturbation} gives, with failure
probability at most $\delta/8$,
\[
\text{(I)}\le L_1\sigma\sqrt{\varepsilon}
= L_1\sqrt{A_c}\,\sigma\sqrt{\frac{u_\delta}{n_{\min}}}.
\]
Lemma~\ref{lem:winsor-concentration} gives, with failure probability at most
$\delta/24$,
\[
\text{(II)}\le L_2\sigma\sqrt{\frac{u_\delta}{n_g}}
\le L_2\sigma\sqrt{\frac{u_\delta}{n_{\min}}}.
\]
Lemma~\ref{lem:winsor-bias} gives deterministically
\[
\text{(III)}\le 4\sigma\sqrt{\varepsilon}
= 4\sqrt{A_c}\,\sigma\sqrt{\frac{u_\delta}{n_{\min}}}.
\]
Hence, with probability at least $1-(\delta/8+\delta/24)=1-\delta/6$,
\begin{equation}
\label{eq:group-bound}
\bigl|\hat\mu_g^{(\mathrm{sep})}-\mu_g\bigr|
\le
C_{\mathrm{grp}}\,\sigma\sqrt{\frac{\log(48/\delta)}{n_{\min}}},
\end{equation}
where
\[
C_{\mathrm{grp}}=L_2+(L_1+4)\sqrt{A_c}.
\]

Then, applying a union bound over $g=0,1$ yields an event of probability at least
$1-2(\delta/6)=1-\delta/3$ on which \eqref{eq:group-bound} holds for both
groups. Thus, on this event, we have
\[
\bigl|\hat\Delta^{(\mathrm{sep})}-\Delta\bigr|
\le
\sum_{g=0}^1\bigl|\hat\mu_g^{(\mathrm{sep})}-\mu_g\bigr|
\le
2C_{\mathrm{grp}}\,\sigma\sqrt{\frac{\log(48/\delta)}{n_{\min}}}.
\]
Set $L_{\mathrm{mean}}=2C_{\mathrm{grp}}$. Since $1-\delta/3\ge1-\delta$, this
proves Theorem~\ref{thm:sep-winsor-mean}.
\end{proof}
