# Supplementary material for: Separate versus Pooled Winsorization in Difference-in-Differences: Bias, Efficiency, and Finite-Sample Guarantees
Source: arXiv:2606.15097 source file (2026-11-14)
Supplement: Supplementary file 4 [file appendix_c_threshold_perturbation.tex]

\subsection{Proof of Lemma~\ref{lem:threshold-perturbation} (Threshold Perturbation)}
\label{app:proof-threshold-perturbation}

Let $u=\log(48/\delta)$ and $A_c=2c^2+\tfrac{8c}{3}$.

Define
\[
\mathcal E_{\mathrm{loc}}
=
\{\alpha^-\le\hat\alpha\le\alpha^+,\ \beta^-\le\hat\beta\le\beta^+\}.
\]
By Lemma~\ref{lem:quantile-localization},
$\Prob(\mathcal E_{\mathrm{loc}})\ge1-\delta/12$.

Define also
\[
\mathcal E_{\mathrm{tail}}
=
\left\{F_m(\alpha^+)\le\varepsilon+\frac{2\varepsilon}{c},
1-F_m(\beta^-)\le\varepsilon+\frac{2\varepsilon}{c}\right\}.
\]
Since $F(\alpha^+)=\varepsilon+\varepsilon/c$, applying the Bernstein inequality for
$\1\{X_i\le\alpha^+\}$ gives
\[
\Prob\!\left(F_m(\alpha^+)>\varepsilon+\frac{2\varepsilon}{c}\right)
\le
\exp\!\left(-\frac{m(\varepsilon/c)^2}{2(\varepsilon+\varepsilon/c)+\tfrac{2}{3}(\varepsilon/c)}\right)
\le e^{-u}=\frac{\delta}{48}.
\]
Likewise, because $\Prob(X>\beta^-)=\varepsilon+\varepsilon/c$, Bernstein inequality for
$\1\{X_i>\beta^-\}$ gives
\[
\Prob\!\left(1-F_m(\beta^-)>\varepsilon+\frac{2\varepsilon}{c}\right)
\le\frac{\delta}{48}.
\]
Hence $\Prob(\mathcal E_{\mathrm{tail}})\ge1-\delta/24$ and with
$\mathcal E=\mathcal E_{\mathrm{loc}}\cap\mathcal E_{\mathrm{tail}}$,
\[
\Prob(\mathcal E)\ge1-\frac{\delta}{8}.
\]

On $\mathcal E_{\mathrm{loc}}$, for any $x\in\R$,
\[
|\phi_{\hat\alpha,\hat\beta}(x)-\phi_{\alpha,\beta}(x)|
\le
|\hat\alpha-\alpha|\,\1\{x\le\max(\hat\alpha,\alpha)\}
+
|\hat\beta-\beta|\,\1\{x\ge\min(\hat\beta,\beta)\}.
\]
Averaging over $X_1,\dots,X_m$ and using the fact that
$\max\{\hat\alpha,\alpha\}\le\alpha^+$,
$\min\{\hat\beta,\beta\}\ge\beta^-$ on $\mathcal E_{\mathrm{loc}}$,
\[
|\hat\mu_{\hat\alpha,\hat\beta}-\hat\mu_{\alpha,\beta}|
\le
|\hat\alpha-\alpha|F_m(\alpha^+)
+
|\hat\beta-\beta|\{1-F_m(\beta^-)\}.
\]
On $\mathcal E_{\mathrm{tail}}$, both empirical tail factors are at most
$\varepsilon(1+2/c)$. On $\mathcal E_{\mathrm{loc}}$,
\[
|\hat\alpha-\alpha|\le|\alpha^+-\alpha^-|,
\qquad
|\hat\beta-\beta|\le|\beta^+-\beta^-|.
\]
By Lemma~\ref{lem:quantile-mean-bound},
\[
|\alpha^+-\alpha^-|\le\frac{2\sigma}{\sqrt{\varepsilon(1-1/c)}},
\qquad
|\beta^+-\beta^-|\le\frac{2\sigma}{\sqrt{\varepsilon(1-1/c)}}.
\]
Therefore, on $\mathcal E$,
\[
|\hat\mu_{\hat\alpha,\hat\beta}-\hat\mu_{\alpha,\beta}|
\le
\frac{4(1+2/c)}{\sqrt{1-1/c}}\,\sigma\sqrt{\varepsilon}
:=L_1\sigma\sqrt{\varepsilon},
\]
with $L_1$ depending only on $c$. Hence
\[
\Prob\!\left(
|\hat\mu_{\hat\alpha,\hat\beta}-\hat\mu_{\alpha,\beta}|
>
L_1\sigma\sqrt{\varepsilon}
\right)
\le\Prob(\mathcal E^c)
\le\frac{\delta}{8},
\]
which is \eqref{eq:threshold-perturbation}. \qed
