# Supplementary material for: Separate versus Pooled Winsorization in Difference-in-Differences: Bias, Efficiency, and Finite-Sample Guarantees
Source: arXiv:2606.15097 source file (2026-11-14)
Supplement: Supplementary file 5 [file appendix_d_winsor_concentration.tex]

\subsection{Proof of Lemma~\ref{lem:winsor-concentration} (Winsorized Mean Concentration)}
\label{app:proof-winsor-concentration}

Let
\[
Z_i=\phi_{\alpha,\beta}(X_i)-\mu_{\alpha,\beta},
\qquad
\bar Z=\frac{1}{m}\sum_{i=1}^m Z_i
=\hat\mu_{\alpha,\beta}-\mu_{\alpha,\beta}.
\]
Then $Z_1,\dots,Z_m$ are i.i.d., $\E(Z_i)=0$,
$\Var(Z_i)=\Var\{\phi_{\alpha,\beta}(X_i)\}\le\Var(X_i)\le\sigma^2$, and
$|Z_i|\le \beta-\alpha$. We define $M = \beta - \alpha$.
By Lemma~\ref{lem:quantile-mean-bound},
\[
|\alpha-\mu|\le\frac{\sigma}{\sqrt\varepsilon},
\qquad
|\beta-\mu|\le\frac{\sigma}{\sqrt\varepsilon},
\]
so $M\le 2\sigma/\sqrt\varepsilon$.

Apply the two-sided Bernstein bound from Lemma~\ref{lem:bernstein-app}:
\[
\Prob(|\bar Z|\ge t)
\le
2\exp\!\left(-\frac{mt^2}{2(\sigma^2+Mt/3)}\right),\qquad t>0.
\]
Set $u=\log(48/\delta)$ and
\[
t=2\sigma\sqrt{\frac{u}{m}}+\frac{4Mu}{3m}.
\]
Write $t=a+b$ with $a=2\sigma\sqrt{u/m}$ and $b=4Mu/(3m)$. Then
$t^2\ge a^2=4\sigma^2u/m$ and $t^2\ge bt=4Mut/(3m)$. Hence
\[
\frac{mt^2}{2}
\ge
2u\sigma^2+\frac{2uMt}{3},
\qquad\text{so}\qquad
\frac{mt^2}{2(\sigma^2+Mt/3)}\ge u,
\]
so
\[
\Prob(|\bar Z|\ge t)\le 2e^{-u}=\frac{\delta}{24}.
\]

It remains to bound $t$ by $\sigma\sqrt{u/m}$. Since
$m\varepsilon\ge A_cu$ with $A_c=2c^2+\tfrac{8c}{3}$,
\[
\frac{4Mu}{3m}
\le
\frac{8\sigma u}{3m\sqrt\varepsilon}
\le
\frac{8\sigma}{3\sqrt{A_c}}\sqrt{\frac{u}{m}}.
\]
Therefore
\[
t\le\left(2+\frac{8}{3\sqrt{A_c}}\right)\sigma\sqrt{\frac{u}{m}}
:=L_2\sigma\sqrt{\frac{u}{m}},
\]
with $L_2$ depending only on $c$. This proves
\eqref{eq:winsor-concentration}. \qed
