# Supplementary material for: Separate versus Pooled Winsorization in Difference-in-Differences: Bias, Efficiency, and Finite-Sample Guarantees
Source: arXiv:2606.15097 source file (2026-11-14)
Supplement: Supplementary file 6 [file appendix_e_winsor_bias.tex]

\subsection{Proof of Lemma~\ref{lem:winsor-bias}}
\label{app:proof-winsor-bias}

Recall that $\alpha = Q_\varepsilon$, $\beta = Q_{1-\varepsilon}$, and
\[
\mu - \mu_{\alpha,\beta}
=
\E\bigl[(X-\alpha)\1\{X<\alpha\}\bigr]
+
\E\bigl[(X-\beta)\1\{X>\beta\}\bigr].
\]
Therefore
\[
|\mu-\mu_{\alpha,\beta}|
\le
\E\bigl[|X-\alpha|\1\{X<\alpha\}\bigr]
+
\E\bigl[|X-\beta|\1\{X>\beta\}\bigr].
\]
We would separately derive upper bound for the two terms.

\medskip
 For the first term, we
write $|X-\alpha| \le |X-\mu| + |\mu-\alpha|$, so
\[
\E\bigl[|X-\alpha|\1\{X<\alpha\}\bigr]
\le
\E\bigl[|X-\mu|\1\{X<\alpha\}\bigr]
+ |\mu-\alpha|\Prob(X<\alpha).
\]
By Cauchy--Schwarz,
\[
\E\bigl[|X-\mu|\1\{X<\alpha\}\bigr]
\le
\sigma\sqrt{\Prob(X<\alpha)}
\le
\sigma\sqrt{\varepsilon}.
\]
By Lemma~\ref{lem:quantile-mean-bound},
$|\mu-\alpha| \le \sigma/\sqrt{\varepsilon}$, and
$\Prob(X<\alpha)\le\varepsilon$, so
\[
|\mu-\alpha|\Prob(X<\alpha)
\le
\frac{\sigma}{\sqrt{\varepsilon}}\cdot\varepsilon
= \sigma\sqrt{\varepsilon}.
\]
Therefore $\E[|X-\alpha|\1\{X<\alpha\}] \le 2\sigma\sqrt{\varepsilon}$.

\medskip
For the second term, applying
the same argument with $\beta = Q_{1-\varepsilon}$ and
$\Prob(X>\beta)\le\varepsilon$ yields
$\E[|X-\beta|\1\{X>\beta\}] \le 2\sigma\sqrt{\varepsilon}$.

\medskip
\noindent Combining two terms together, 
\[
|\mu_{\alpha,\beta} - \mu|
\le
4\sigma\sqrt{\varepsilon},
\]
which is exactly \eqref{eq:winsor-bias}.

% --------------------------------------------------
%  APPENDIX E: Quantile--mean distance proof
% --------------------------------------------------
