# Supplementary material for: Separate versus Pooled Winsorization in Difference-in-Differences: Bias, Efficiency, and Finite-Sample Guarantees
Source: arXiv:2606.15097 source file (2026-11-14)
Supplement: Supplementary file 7 [file appendix_f_quantile_mean.tex]

\subsection{Proof of Lemma~\ref{lem:quantile-mean-bound}}
\label{app:proof-quantile-mean}

Fix $p\in(0,1)$.
Use the definition of quantile $Q_p = \inf\{x\in\R:F(x)\ge p\}$.

\medskip
\noindent Case (1): If $Q_p \le \mu$,
set $t = \mu - Q_p \ge 0$. Then
\[
p \le \Prob(X\le Q_p) \le \Prob(X\le\mu-t) \le \Prob(|X-\mu|\ge t)
\le \frac{\sigma^2}{t^2},
\]
where the last step is Chebyshev's inequality. Hence $t \le \sigma/\sqrt{p}$.

\medskip
\noindent Case (2): If $Q_p \ge \mu$,
set $t = Q_p - \mu \ge 0$. Then
\[
1-p \le \Prob(X\ge Q_p) \le \Prob(X\ge\mu+t) \le \Prob(|X-\mu|\ge t)
\le \frac{\sigma^2}{t^2},
\]
so $t \le \sigma/\sqrt{1-p}$.

\medskip
\noindent Combining
$|Q_p - \mu| \le \sigma/\sqrt{\min\{p,1-p\}}$. \qed

% --------------------------------------------------
%  APPENDIX F: Pooled balanced impossibility proof
% --------------------------------------------------
