# Supplementary material for: Separate versus Pooled Winsorization in Difference-in-Differences: Bias, Efficiency, and Finite-Sample Guarantees
Source: arXiv:2606.15097 source file (2026-11-14)
Supplement: Supplementary file 8 [file appendix_g_pooled_impossibility.tex]

\section{Proof of Theorem~\ref{thm:pooled-mean-impossibility} (Deterministic Pooled Impossibility)}
\label{app:proof-pooled-impossibility}

Throughout this proof, we fix a balanced group size $n_0=n_1=m$ and let
\[
n=2m,\qquad
\hat\alpha=\hat\alpha_n^{(\mathrm{pool})}=Z_{(\lceil 2m\eps\rceil)},\qquad
\hat\beta=\hat\beta_n^{(\mathrm{pool})}=Z_{(\lceil 2m(1-\eps)\rceil)}.
\]
And we set $k=\lceil 2m\eps\rceil,~ t=\lfloor 2m\eps\rfloor.$ 

To prove Theorem~\ref{thm:pooled-mean-impossibility}, we construct distributions
$P_0,P_1\in \mathcal{P}(\sigma^2)$ under which the lower bound in
\eqref{eq:pooled-mean-impossibility} holds for every possible choice of the
winsorization rule $\eps$. Since $\eps$ may induce different degrees of truncation, we divide the analysis
into two regimes. Let $u$ denote the number of observations winsorized on one
side of the distribution, as determined by the rule $\eps$. We define the weak
winsorization regime as the case where $u \le \log(2/\delta)+1$, and the strong
winsorization regime as the case where $u > \log(2/\delta)+1$. For each regime, we construct a different pair of distributions under which the
lower bound in \eqref{eq:pooled-mean-impossibility} holds.

In the following subsection, we will first state and prove the supporting lemmas for the proof of Theorem~\ref{thm:pooled-mean-impossibility}:

\subsection{Preparatory Lemmas for Theorem~\ref{thm:pooled-mean-impossibility}}

\begin{lemma}\label{lem:pool-sep}
Fix $r>0$, $M\ge0$, and $D>M+2r$. If $Y_{0,i}\in[-D-r,-D+r]$, $Y_{1,i}\in[-M-r,\infty)\ \text{a.s.},$
then we have
\[
\max_{1\le i\le m}Y_{0,i}<\min_{1\le i\le m}Y_{1,i} ~ \text{a.s.}.
\]
\end{lemma}

\begin{proof}
Immediate from $-D+r<-M-r\le\min_iY_{1,i}$ and $\max_iY_{0,i}\le -D+r$.
\end{proof}

\begin{lemma}\label{lem:pool-index}
We define the event
\[
\mathsf{Sep}=\{\max_{1 \leq i \leq m}Y_{0,i}<\min_{1 \leq i \leq m}Y_{1,i}\}. 
\]
On this event, we have
\[
\hat\alpha=Y_{0,(k)},\qquad
\hat\beta=Y_{1,(m-t)}.
\]
\end{lemma}

\begin{proof}
On $\mathsf{Sep}$, pooled order statistics split by group: the first $m$ are group~0 and the
last $m$ are group~1. Hence $\hat\alpha=Z_{(k)}=Y_{0,(k)}$. Also
\[
\hat\beta
=
Z_{(\lceil 2m(1-\eps)\rceil)}
=
Y_{1,(\lceil 2m(1-\eps)\rceil-m)}
=
Y_{1,(m-t)},
\]
because $\lceil 2m(1-\eps)\rceil=2m-\lfloor 2m\eps\rfloor=2m-t$.
\end{proof}

\begin{lemma}\label{lem:pool-binom}
If $X\sim\mathrm{Bin}(m,p)$ and $mp\in\mathbb{Z}$, then
\[
\Prob(X\le mp)\ge\tfrac12.
\]
\end{lemma}

\begin{proof}
A classical fact for binomial distribution states that any median of
$\mathrm{Bin}(m,p)$ lies in $\{\lfloor mp\rfloor,\lceil mp\rceil\}$. If $mp$ is an integer,
this set is $\{mp\}$, so $mp$ is a median.
\end{proof}

\begin{lemma}[Log comparison]\label{lem:pool-log}
For every $\delta\in(0,\tfrac14)$, we have that
\[
\log\frac1{2\delta}\ge \frac13\log\frac2\delta.
\]
\end{lemma}

\begin{proof}
Let $a=\log(1/(2\delta))$. Since $\delta\le1/4$, $a\ge\log 2$, and
\[
\log\frac2\delta=\log\!\left(4\cdot\frac1{2\delta}\right)=2\log2+a\le3a.
\]
Thus the inequality holds.
\end{proof}
With the above lemmas, we could show that if the winsorization rule is weak (i.e., $u\le \log(2/\delta) + 1$), we have the following finite-sample lower bound for one-sided winsorization. 
\begin{lemma}\label{lem:pool-undertrim}
Set $L=1/4$. For any $m\ge1$,
$\delta\in(0,\tfrac14)$, and integer $u\in\{0,\dots,m-1\}$ with
$u\le \log(2/\delta)+1$, there exists a continuous distribution 
$P\in\mathcal{P}(\sigma^2)$ with mean $\mu$ such that the one-sided
winsorization estimator
\[
\hat\mu_u=\frac1m\sum_{i=1}^m\min\{X_i,X_{(m-u)}\},\qquad X_i\stackrel{\mathrm{i.i.d.}}{\sim}P,
\]
satisfies
\[
\Prob\!\left(
\left|\hat\mu_u-\mu\right|>
L\sigma\sqrt{\frac{\log(2/\delta)}{m}}
\right)>\delta.
\]
\end{lemma}

\begin{proof}
Let
\[
q=1-(2\delta)^{1/m},\quad s=1-q,\quad
r=\min\!\left\{\frac{\sigma}{100},\frac{\sigma}{40}\sqrt{\frac{\log(2/\delta)}{m}}\right\},
\]
and define $X$ to be the mixture of two uniform distributions
\[
X\sim (1-q)\,\mathrm{Unif}[-r,r]+q\,\mathrm{Unif}[B-r,B+r],\qquad
B=\sqrt{\frac{\sigma^2-r^2/3}{q(1-q)}}.
\]
Then $X$ is continuously distributed with mean
\[
\mu=\E[X] = qB=\sqrt{\sigma^2-r^2/3}\,\sqrt{\frac{q}{1-q}}.
\]
and variance
\[
\Var(X)=q(1-q)B^2+r^2/3=\sigma^2.
\]

Let $N_+ = \sum_{i=1}^m \mathbb{I}(X_i \in [B-r, B+r])$ be the number of observations falling into the upper-bump component $[B-r, B+r]$, so that $N_+\sim\mathrm{Bin}(m,q)$, and set $\mathsf{A} = \{N_+=0\}$. Then
\[
\Prob(\mathsf{A})=(1-q)^m=s^m=2\delta>\delta.
\]
On $\mathsf{A}$, all observations lie in $[-r,r]$, hence $|\hat\mu_u|\le r$ for every
$u\in\{0,\dots,m-1\}$ and
\[
|\hat\mu_u-\mu|\ge \mu-r.
\]

Write $x=\log(1/(2\delta))/m$. Since $q/(1-q)=e^x-1\ge x$ and by
Lemma~\ref{lem:pool-log},
\[
\mu
\ge
\frac{99}{100}\sigma\sqrt{\frac{1}{3}\frac{\log(2/\delta)}{m}}.
\]
Also $r\le\frac1{40}\sigma\sqrt{\log(2/\delta)/m}$. Therefore
\[
\mu-r
\ge
\left(\frac{99}{100\sqrt3}-\frac1{40}\right)\sigma\sqrt{\frac{\log(2/\delta)}{m}}
>
\frac14\sigma\sqrt{\frac{\log(2/\delta)}{m}}.
\]
Thus on $\mathsf{A}$,
\[
|\hat\mu_u-\mu|>
L\sigma\sqrt{\frac{\log(2/\delta)}{m}},
\qquad L=\frac14
\]
.
\end{proof}

\subsection{Proof of Theorem~\ref{thm:pooled-mean-impossibility}}

\begin{proof}
Fix $\sigma^2>0$, a deterministic rule
$\eps:\mathbb{N}\times(0,\tfrac14)\to(0,\tfrac12)$, and arbitrary $m\ge1$,
$\delta\in(0,\tfrac14)$. Let
\[
\tau_{m,\delta}=\frac18\,\sigma\sqrt{\frac{\log(2/\delta)}{m}}.
\]
Since $\eps\in(0,1/2)$, $t=\lfloor2m\eps\rfloor\in\{0,\dots,m-1\}$. We consider the following two regimes that include all the possible deterministic rules. In both regimes, we will show that there exists $P_0,P_1\in \mathcal{P}(\sigma^2)$ such that:
\[
\Prob\!\left(
\left|\hat\Delta^{(\mathrm{pool})}-\Delta\right|>\tau_{m,\delta}
\right)>\delta.
\]

\medskip\noindent\textit{Regime 1: weak winsorization.}
Assume
\[
t\le \log(2/\delta)+1.
\]
Apply Lemma~\ref{lem:pool-undertrim} with $u=t$, and let $P_1$ denote the distribution defined in Lemma~\ref{lem:pool-undertrim} with mean $\mu_1$.

Set
\[
\rho_0=\frac{1}{256}\sigma\sqrt{\frac{\log(2/\delta)}{m}},\qquad
P_0=\mathrm{Unif}[-D_0-\rho_0,-D_0+\rho_0],
\]
where $D_0$ is chosen large enough such that
\[
-D_0+\rho_0<\inf\mathrm{supp}(P_1).
\]
Then $\max_iY_{0,i}<\min_iY_{1,i}$ almost surely, so lower clipping never affects group~1.
Also $\mu_0=-D_0$ and therefore $\Delta=\mu_1-\mu_0=\mu_1+D_0$. Define the one-sided winsorized mean $\hat\mu_t=\frac1m\sum_{i=1}^m\min\{Y_{1,i},Y_{1,(m-t)}\}$,
by Lemma~\ref{lem:pool-index}:
\[
\frac1m\sum_{i=1}^m\phi_{\hat\alpha,\hat\beta}(Y_{1,i})-\mu_1
=
\hat\mu_t-\mu_1.
\]
Moreover,
\[
\left|
\frac1m\sum_{i=1}^m\phi_{\hat\alpha,\hat\beta}(Y_{0,i})-\mu_0
\right|
\le
\rho_0
=
\frac1{256}\sigma\sqrt{\frac{\log(2/\delta)}{m}}.
\]
If we set $L = 1/4$, applying Lemma \ref{lem:pool-undertrim}, we know that the following event has probability $>\delta$:
\[
\left\{|\hat\mu_t-\mu_1|>
L\sigma\sqrt{\frac{\log(2/\delta)}{m}}\right\}.
\]
Thus, on this event, by triangle inequality, we have
\[
\left|\hat\Delta^{(\mathrm{pool})}-\Delta\right|
\ge
\left(L-\frac1{256}\right)\sigma\sqrt{\frac{\log(2/\delta)}{m}}
>
\frac18\,\sigma\sqrt{\frac{\log(2/\delta)}{m}}
=
\tau_{m,\delta}.
\]
And this event has probability $>\delta$:
\[
\Prob\!\left(
\left|\hat\Delta^{(\mathrm{pool})}-\Delta\right|>\tau_{m,\delta}
\right)>\delta.
\]

\medskip\noindent\textit{Regime 2: strong winsorization.}
Assume
\[
t>\log(2/\delta)+1.
\]
Then $t\ge1$. Set
\[
p=\frac{t}{m}\in(0,1),\qquad
r=\min\!\left\{\frac{\sigma}{100},\frac{\sigma}{100}\sqrt{\frac{\log(2/\delta)}{m}}\right\},
\qquad
\sigma_-=\sqrt{\sigma^2-r^2/3},
\]
\[
M=\sigma_-\sqrt{\frac{p}{1-p}},\qquad
x_+=\frac{1-p}{p}M.
\]
Define
\[
P_1=(1-p)\,\mathrm{Unif}[-M-r,-M+r]+p\,\mathrm{Unif}[x_+-r,x_++r].
\]
Then $P_1$ is continuous, $\E(Y_{1,1})=0$, and
\[
\Var(Y_{1,1})=(1-p)M^2+px_+^2+\frac{r^2}{3}
=
\sigma_-^2+\frac{r^2}{3}
=
\sigma^2.
\]
Also, from $p>\log(2/\delta)/m$ and $\sigma_-\ge(99/100)\sigma$,
\[
M>\frac{99}{100}\sigma\sqrt{\frac{\log(2/\delta)}{m}}.
\]
Combining this with $r\le(\sigma/100)\sqrt{\log(2/\delta)/m}$ yields
\[
\frac{r}{M}
<
\frac{(\sigma/100)\sqrt{\log(2/\delta)/m}}
     {(99/100)\sigma\sqrt{\log(2/\delta)/m}}
=
\frac1{99}
\le
\frac18,
\]
so $r\le M/8$.

Let
\[
D=M+x_++4r,\qquad
P_0=\mathrm{Unif}[-D-r,-D+r].
\]
Then $P_0$ is continuous and $\Var(Y_{0,1})=r^2/3\le\sigma^2$, so
$P_0\in\mathcal{P}(\sigma^2)$. Since $D>M+2r$, Lemma~\ref{lem:pool-sep}
implies $\mathsf{Sep}$ holds almost surely.

Let $N_+ = \sum_{i=1}^m \mathbb{I}(Y_{1,i} \in [x_+-r, x_++r])$ be the number of group-1 observations falling into the upper-bump component; then $N_+\sim\mathrm{Bin}(m,p)$. Define
\[
\mathsf{E}=\{N_+\le t\}.
\]
Because $mp=t\in\mathbb Z$, Lemma~\ref{lem:pool-binom} gives
\[
\Prob(\mathsf{E})\ge\tfrac12>\delta.
\]
Similarly, define $N_-=m-N_+$ to be the number of observations falling into the lower-bump component, on $\mathsf{E}$ and $\mathsf{Sep}$, Lemma~\ref{lem:pool-index} gives
$\hat\beta=Y_{1,(m-t)}$. Since $m-t \le m-N_+ = N_-$, the order statistic $Y_{1,(m-t)}$ lies in the
lower-bump component $[-M-r, -M+r]$, hence $\hat\beta\le -M+r$. Also
$\hat\alpha=Y_{0,(k)}\le -D+r<-M-r\le\min_iY_{1,i}$, so lower clipping does not act on group~1.
Therefore
\[
\frac1m\sum_{i=1}^m\phi_{\hat\alpha,\hat\beta}(Y_{1,i})\le -M+r,\qquad
\frac1m\sum_{i=1}^m\phi_{\hat\alpha,\hat\beta}(Y_{0,i})\ge -D-r.
\]
Hence, with $\Delta=\mu_1-\mu_0=0-(-D)=D$,
\[
\left|\hat\Delta^{(\mathrm{pool})}-\Delta\right|
\ge
M-2r
\ge
\frac34 M
\ge
\frac{297}{400}\sigma\sqrt{\frac{\log(2/\delta)}{m}}
>
\frac18\sigma\sqrt{\frac{\log(2/\delta)}{m}}
=
\tau_{m,\delta}.
\]
Thus, on $\mathsf{E}$,
\[
\left|\hat\Delta^{(\mathrm{pool})}-\Delta\right|>\tau_{m,\delta},
\]
and since $\Prob(\mathsf{E})>\delta$,
\[
\Prob\!\left(
\left|\hat\Delta^{(\mathrm{pool})}-\Delta\right|>\tau_{m,\delta}
\right)>\delta.
\]

Since Regimes 1 and 2 are exhaustive, we have completed the proof.
\end{proof}
