# Supplementary material for: Separate versus Pooled Winsorization in Difference-in-Differences: Bias, Efficiency, and Finite-Sample Guarantees
Source: arXiv:2606.15097 source file (2026-11-14)
Supplement: Supplementary file 9 [file appendix_i_multigroup_contrast_proof.tex]

\section{Proof of Theorem~\ref{thm:sep-winsor-multigroup}}
\label{app:proof-sep-winsor-multigroup}

\begin{proof}
The proof of Theorem~\ref{thm:sep-winsor-multigroup} follows as a direct
extension of Theorem~\ref{thm:sep-winsor-mean}. We therefore only sketch the key
steps. Set
\[
\bar\delta=\frac{\delta}{K},
\qquad
u_\delta=\log\!\left(\frac{48K}{\delta}\right)
=\log\!\left(\frac{48}{\bar\delta}\right),
\qquad
A_c=2c^2+\frac{8c}{3},
\]
and $\varepsilon=A_cu_\delta/n_{\min}$.

Step 1. Fix any group $g\in\{0,\dots,K-1\}$. Define
$\alpha_g=Q_\varepsilon^{(g)}$ and $\beta_g=Q_{1-\varepsilon}^{(g)}$. As in
Appendix~\ref{app:proof-sep-winsor-main},
\[
\bigl|\hat\mu_g^{(\mathrm{sep})}-\mu_g\bigr|
\le
\underbrace{\bigl|\hat\mu_{\hat\alpha_g,\hat\beta_g}-\hat\mu_{\alpha_g,\beta_g}\bigr|}_{\text{(I)}}
+
\underbrace{\bigl|\hat\mu_{\alpha_g,\beta_g}-\mu_{\alpha_g,\beta_g}\bigr|}_{\text{(II)}}
+
\underbrace{\bigl|\mu_{\alpha_g,\beta_g}-\mu_g\bigr|}_{\text{(III)}}.
\]
% Since $n_g\ge n_{\min}$, we have
% $n_g\varepsilon\ge A_cu_\delta=A_c\log(48/\bar\delta)$, so
% Lemmas~\ref{lem:quantile-localization}--\ref{lem:winsor-concentration} apply
% with confidence parameter $\bar\delta$. 
Therefore, applying Lemmas~\ref{lem:threshold-perturbation}--\ref{lem:winsor-concentration} to $\text{(I)}-\text{(II)}$, we have that,
\[
\text{(I)}
\le
L_1\sigma\sqrt{\varepsilon}
=
L_1\sqrt{A_c}\,\sigma\sqrt{\frac{u_\delta}{n_{\min}}},
\]
\[
\text{(II)}
\le
L_2\sigma\sqrt{\frac{u_\delta}{n_g}}
\le
L_2\sigma\sqrt{\frac{u_\delta}{n_{\min}}},
\]
with failure probability at
most $\bar\delta/8+\bar\delta/24=\bar\delta/6$. Then, applying Lemma~\ref{lem:winsor-bias} to \text{(III)}, we have that
\[
\text{(III)}
\le
4\sigma\sqrt{\varepsilon}
=
4\sqrt{A_c}\,\sigma\sqrt{\frac{u_\delta}{n_{\min}}}
\]
holds deterministically. Hence, for
$C_{\mathrm{grp}}=L_2+(L_1+4)\sqrt{A_c}$,
\begin{equation}
\label{eq:multigroup-group-bound}
\Prob\!\left(
  \bigl|\hat\mu_g^{(\mathrm{sep})}-\mu_g\bigr|
  \le
  C_{\mathrm{grp}}\,
  \sigma\sqrt{\frac{u_\delta}{n_{\min}}}
\right)
\ge
1-\frac{\bar\delta}{6}.
\end{equation}

Step 2. Apply a union bound to \eqref{eq:multigroup-group-bound} over all
$g=0,\dots,K-1$. Then, with probability at least
$1-K\bar\delta/6=1-\delta/6$, we have simultaneously
\[
\bigl|\hat\mu_g^{(\mathrm{sep})}-\mu_g\bigr|
\le
C_{\mathrm{grp}}\,
\sigma\sqrt{\frac{u_\delta}{n_{\min}}}
\quad
\text{for all }g.
\]

Step 3. On this event,
\[
\bigl|\hat\Delta^{(\mathrm{sep})}-\Delta\bigr|
=
\left|\sum_{g=0}^{K-1} c_g\bigl(\hat\mu_g^{(\mathrm{sep})}-\mu_g\bigr)\right|
\le
\sum_{g=0}^{K-1}|c_g|\,\bigl|\hat\mu_g^{(\mathrm{sep})}-\mu_g\bigr|
\le
K\,
C_{\mathrm{grp}}\,
\sigma\sqrt{\frac{u_\delta}{n_{\min}}}.
\]
The last inequality uses $|c_g|\le 1$ for all $g$, hence
$\sum_{g=0}^{K-1}|c_g|\le K$. Set $L=C_{\mathrm{grp}}$. Since
$1-\delta/6\ge1-\delta$,
\eqref{eq:multigroup-contrast-bound} follows.
\end{proof}
