# Supplementary material for: Separate versus Pooled Winsorization in Difference-in-Differences: Bias, Efficiency, and Finite-Sample Guarantees
Source: arXiv:2606.15097 source file (2026-11-14)
Supplement: Supplementary file 10 [file appendix_j_additional_simulation.tex]

\section{Additional simulation studies}
\label{app:additional-simulation}

In this appendix, we further examine the sensitivity of the separate and pooled
winsorization estimators to the choice of the winsorization level $\varepsilon$. The
main simulation study uses the theoretically calibrated value of $\varepsilon$ from
Theorem~\ref{thm:sep-winsor-mean}. Here, we vary $\varepsilon$ from $0.005$ to $0.30$, and compare the behavior of the separate and pooled
winsorized estimators in terms of bias, RMSE,
and containment in the theoretical 95\% CLT interval for the naive mean-difference estimator.

Figure~\ref{fig:eps_balanced}
summarizes the results for the balanced group design. The left column of Figure~\ref{fig:eps_balanced}
shows that separate winsorization has negligible absolute bias across the entire range
of $\varepsilon$ values. In contrast, pooled winsorization becomes increasingly biased
as $\varepsilon$ grows, under all of the five distributions considered. The middle column of Figure~\ref{fig:eps_balanced} shows a similar pattern for RMSE. Separate
winsorization is stable across the range of $\varepsilon$ values. Pooled winsorization also performs reasonably when $\varepsilon$ is below 0.05, but its RMSE increases rapidly as $\varepsilon$ increases. The right column of Figure~\ref{fig:eps_balanced} further shows that separate winsorization generally maintains high containment, while pooled
winsorization can have substantially lower containment when the winsorization level
is above 0.05. Together, these results suggest that the empirical advantage
of separate winsorization is not specific to the theoretically calibrated choice of
$\varepsilon$. Finally, Figure~\ref{fig:eps_imbalanced} reports the corresponding results for the imbalanced group design, and the results are qualitatively  similar to those in the balanced group design. 

%\clearpage

\begin{figure}[h]
\figuresize{.8}
\figurebox{20pc}{25pc}{}[Figures/fig_eps_balanced]
\caption{Sensitivity of absolute bias (the left column), RMSE (the middle column), and theoretical-CLT containment (the right column) to the winsorization level under the balanced group design. The vertical dotted line marks the theoretically calibrated winsorization level at $\varepsilon=0.092$; in the containment panels, the horizontal dotted line marks the nominal 95\% level.}
\label{fig:eps_balanced} 
\end{figure}

\begin{figure}[h]
\figuresize{.8}
\figurebox{20pc}{25pc}{}[Figures/fig_eps_imbalanced]
\caption{Sensitivity of absolute bias (the left column), RMSE (the middle column), and theoretical-CLT containment (the right column) to the winsorization level under the imbalanced group design. The vertical dotted line marks the theoretically calibrated winsorization level at $\varepsilon=0.092$; in the containment panels, the horizontal dotted line marks the nominal 95\% level.}
\label{fig:eps_imbalanced} 
\end{figure}
